# Supplementary material for: Real-time ab initio simulation of inelastic electron scattering using the exact, density functional, and alternative approaches
Source: arXiv:2004.01802 source file (2020-04-03)
Supplement: Supplementary file 1 [file supplement.pdf]

# Supplemental material for "Real-time ab initio simulation of inelastic electron scattering using the exact, density functional, and alternative approaches"

Yeonghun Lee, Xiaolong Yao, Massimo V. Fischetti, and Kyeongjae Cho*

*Department of Materials Science and Engineering,*
*University of Texas at Dallas, Richardson, TX 75080, USA*
*kjcho@utdallas.edu

(Dated: April 3, 2020)

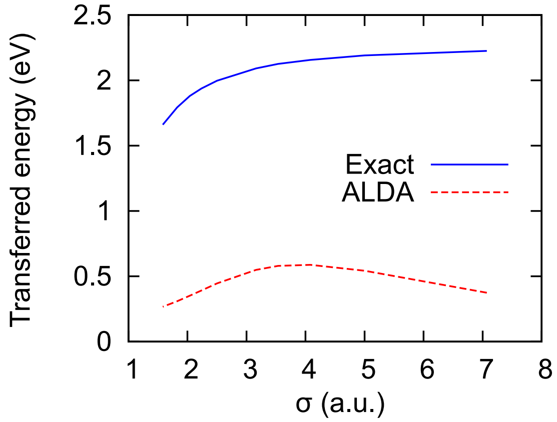


FIG. S1. Transferred energy as a function of the $\sigma$, which is a width of the Gaussian wave packet. These are calculated by using the spin-unpolarized exact solution (solid line) and TDDFT with spin-unpolarized ALDA (dashed line). The incoming wave packet parameters except for $\sigma$ are the same as in Figs. 1(a–c). In the exact solution, the transferred energy monotonically increases as $\sigma$ increases and then saturates. Throughout the paper, we use $\sigma = 2.236$ a.u., around which the ALDA exhibits similar tendency to the exact solution.

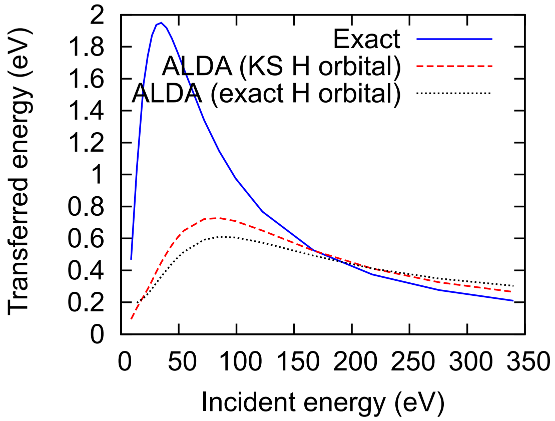


FIG. S2. In the TDDFT, the initial orbital of the bound electron can be given in two different ways: the exact orbital of the 1D hydrogen shown in Fig. 2(a) or the corresponding KS orbital shown in Fig. 2(b). The small deviation of the energy transferred is attributed to the similar electron density profile between the KS and exact hydrogen orbitals. These are results of spin-unpolarized calculation.

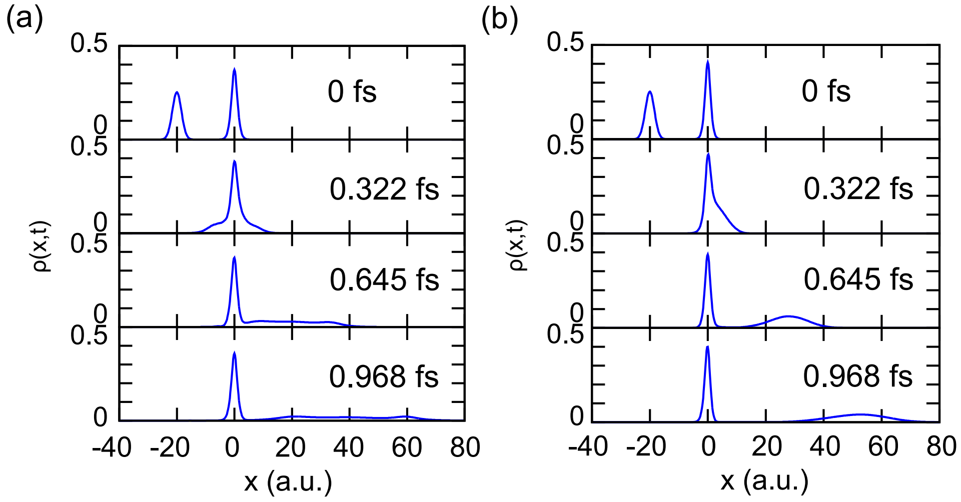


FIG. S3. Same as Fig. 1(a), but TDDFT with spin-unpolarized (a) ALDA and (b) SIC are exploited. The incident wave packet parameters except for the initial spin state are the same as in Figs. 1(a–c).

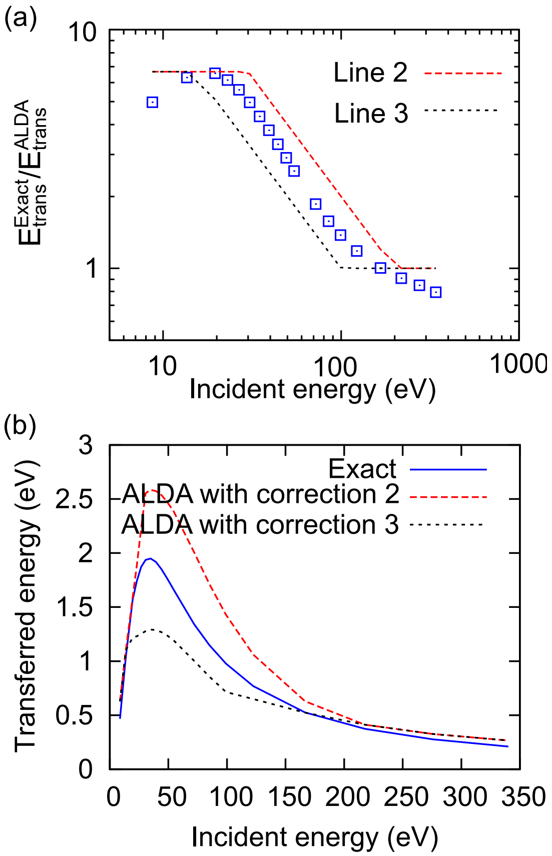


FIG. S4. Same as Fig. 7, but the upper and lower turning points in the relationship $E_{trans}^{Exact}/E_{trans}^{ALDA}$ are different. (a) The line 2 (dashed line) is a function expressed as: $y = 200/30$ for $x < 30$; $y = 200/x$ for $30 \le x < 200$; $y = 200/200$ for $200 \le x$. The line 3 (dotted line) is a function expressed as: $y = 100/15$ for $x < 15$; $y = 100/x$ for $15 \le x < 100$; $y = 100/100$ for $100 \le x$. (b) The corrections 2 and 3 adopt the lines 2 and 3, respectively.
